# Supplementary material for: The Method of Harmonic Balance for the Giesekus Model under Oscillatory Shear
Source: arXiv:2301.11131 source file (2023-01-26)
Supplement: Supplementary file 1 [file Supplementary_material.pdf]

# Supplementary Material

## The Method of Harmonic Balance for Giesekus Model under Oscillatory Shear

Shivangi Mittal[1], Yogesh M. Joshi[1], and Sachin Shanbhag[2,*]

[1]Department of Chemical Engineering, Indian Institute of Technology Kanpur, India
[2]Department of Scientific Computing, Florida State University, Tallahasee, Florida, USA

## Contents

**1 Nomenclature** **S2**

**2 Deriving the Harmonic Balance equation system** **S4**

# 1 Nomenclature

A list of symbols used in the paper is provided below.

| Description | Symbol |
|---|---|
| Anisotropy parameter in Giesekus model | $\alpha$ |
| Shear stress | $\sigma_{12}$ |
| First normal stress | $\sigma_{11}$ |
| Second normal stress | $\sigma_{22}$ |
| First normal stress difference | $N_1 = \sigma_{11} - \sigma_{22}$ |
| Second normal stress difference | $N_2 = \sigma_{22} - \sigma_{33}$ |
| Deborah number | $\mathrm{De} = \lambda\omega$ |
| Weissenberg number | $\mathrm{Wi} = \lambda\omega\gamma_0$ |
| Sine and cosine Fourier coefficients of $\sigma_{11}$ | $P'_n, P''_n$ |
| Sine and cosine Fourier coefficients of $\sigma_{22}$ | $Q'_n, Q''_n$ |
| Sine and cosine Fourier coefficients of $\sigma_{12}$ | $G'_n, G''_n$ |
| Power series coefficients for $\sigma_{12}$ | $G'_{ij}, G''_{ij}$ |
| Sine and cosine Fourier coefficients of $N_1$ | $F'_n, F''_n$ |
| Power series coefficients for $N_1$ | $F'_{ij}, F''_{ij}$ |
| Sine and cosine Fourier coefficients of $N_2$ | $S'_n, S''_n$ |
| Power series coefficients for $N_2$ | $S'_{ij}, S''_{ij}$ |
| $k$th Fourier coefficient of $y(t)$ | $Y_k$ |
| Number of harmonics | $H$ |
| Harmonic approximation of $y(t)$ with $H$ harmonics | $y_H$ |
| Matrix of Fourier coefficients for $y_H$ | $\boldsymbol{M}$ |
| Column vector of Fourier functions, eqn. (22) | $\boldsymbol{h}(\omega t)$ |
| scalar/column vector of residuals with truncation upto $H$ harmonics | $r_H$/$\boldsymbol{r}_H$ |
| Matrix of Fourier coefficients of the residuals $\boldsymbol{r}_H$ | $\boldsymbol{R}$ |
| Diagonal matrix of constant coefficients for the ODE system | $\boldsymbol{K}$ |
| Column vector of nonlinear terms in ODE system, eqn. (32) | $\boldsymbol{f}_{nl}$ |
| Column vector of external forcing terms in ODE system, eqn. (33) | $\boldsymbol{f}_{ex}$ |
| Matrix of Fourier coefficients for $\boldsymbol{f}_{nl}$ | $\boldsymbol{F}_{nl}$ |
| Matrix of Fourier coefficients for $\boldsymbol{f}_{ex}$ | $\boldsymbol{F}_{ex}$ |
| Infinity norm of difference between true and HB solutions | $\xi$ |
| Convergence decay coefficient | $m$ |
| Complex Fourier coefficient for the $k$th harmonic of $\sigma_{11}$ | $A_{2k}$ |
| Complex Fourier coefficient for the $k$th harmonic of $\sigma_{22}$ | $B_{2k}$ |
| Complex Fourier coefficient for the $k$th harmonic of $\sigma_{12}$ | $C_{2k+1}$ |

| Description | Symbol |
|---|---|
| $k$th element of residual vector $\boldsymbol{R}^{ij}$ corresponding to ODE for $\sigma_{ij}$ | $R_k^{ij}$ |
| Dimensionless stress vector | $\tilde{\boldsymbol{\sigma}} = \boldsymbol{\sigma}/G\lambda\omega\gamma_0$ |
| Dimensionless time | $\tilde{t} = t/\lambda$ |
| Dimensionless shear rate | $\tilde{\dot{\gamma}} = \dot{\gamma}/\gamma_0\omega$ |
| Residual terms corresponding to $\sigma_{11}, \sigma_{22}$ and $\sigma_{12}$ in IVP | $r_{11}, r_{22}, r_{12}$ |
| Euclidean norm or the root mean square residual | $\epsilon_r$ |

Table S1: Summary of symbols and notations used

# 2 Deriving the Harmonic Balance equation system

In this section, we describe the derivation of the harmonic balance system of nonlinear equations for the Giesekus model subjected to large amplitude oscillatory shear. We start with the Giesekus model equations with $\eta_s = 0$.

$$\frac{d\sigma_{11}}{dt} + \frac{\sigma_{11}}{\lambda} + \frac{\alpha}{\lambda G}\left(\sigma_{11}^2 + \sigma_{12}^2\right) - 2\dot{\gamma}\sigma_{12} = 0, \tag{1}$$

$$\frac{d\sigma_{22}}{dt} + \frac{\sigma_{22}}{\lambda} + \frac{\alpha}{\lambda G}\left(\sigma_{22}^2 + \sigma_{12}^2\right) = 0, \tag{2}$$

$$\frac{d\sigma_{12}}{dt} + \frac{\sigma_{12}}{\lambda} + \frac{\alpha}{\lambda G}\left(\sigma_{11} + \sigma_{22}\right)\sigma_{12} - \sigma_{22}\dot{\gamma} - G\dot{\gamma} = 0. \tag{3}$$

Since $\sigma_{33}$ has a trivial solution, it is not included in the equation system. The three variables $(\sigma_{11,}\sigma_{22}, \sigma_{12})$ can be represented as a truncated Fourier series with $H$ odd harmonics, i.e. $2H$ terms in shear stress and $(2H-1)$ terms in normal stress expansion.

$$\boldsymbol{\sigma}_H(t) = \begin{bmatrix} \sigma_{11,H} \\ \sigma_{22,H} \\ \sigma_{12,H} \end{bmatrix} = \begin{bmatrix} \sum_{k=-(H-1)}^{(H-1)} A_{2k} e^{i2k\omega t} \\ \sum_{k=-(H-1)}^{(H-1)} B_{2k} e^{i2k\omega t} \\ \sum_{k=-H}^{(H-1)} C_{2k+1} e^{i(2k+1)\omega t} \end{bmatrix}. \tag{4}$$

In addition, for an oscillatory shear deformation, we know

$$\dot{\gamma} = \gamma_0\omega\cos(\omega t) = \frac{\gamma_0\omega}{2}\left(e^{i\omega t} + e^{-i\omega t}\right). \tag{5}$$

When the truncated Fourier representations in eqn. (4) are plugged in the Giesekus model equation system (1) – (3), the right hand side is not identically zero. Let this residual term be $\boldsymbol{r}_H$. $\boldsymbol{r}_H$ inherits periodicity from the forcing function, and can also be represented as a Fourier series,

$$\boldsymbol{r}_H(t) = \begin{bmatrix} r_H^{11} \\ r_H^{22} \\ r_H^{12} \end{bmatrix} = \begin{bmatrix} \sum_{k=-(H-1)}^{(H-1)} R_k^{11} e^{i2k\omega t} \\ \sum_{k=-(H-1)}^{(H-1)} R_k^{22} e^{i2k\omega t} \\ \sum_{k=-H}^{(H-1)} R_k^{12} e^{i(2k+1)\omega t} \end{bmatrix}. \tag{6}$$

The goal of HB is to minimize this residual by setting the individual Fourier coefficients $(R_k^{11}, R_k^{22}, R_k^{12})$ to zero. Thus, by substituting eqn. (4) in eqn. (1) – (3) and equating to (6), we obtain a system of nonlinear equations which have to be solved for $A_{2k}$, $B_{2k}$ and $C_{2k+1}$.

To resolve the quadratic terms encountered in the equation system viz. $\sigma_{11}^2, \sigma_{22}^2, \sigma_{12}^2$ and $\sigma_{12}(\sigma_{11} + \sigma_{22})$, we use the convolution theorem. This theorem states that the product $x(t)$ of two Fourier

series $u(t)$ and $v(t)$ which are given by

$$u(t) = \sum_{m=-M}^{M} U_m e^{im\omega t}$$

and

$$v(t) = \sum_{n=-N}^{N} V_n e^{in\omega t},$$

is also a truncated Fourier series of order $M + N$ given by,

$$x(t) = u(t)v(t) = \sum_{m=-M}^{M} \sum_{n=-N}^{N} U_m V_n e^{i(m+n)\omega t} = \sum_{k=-(M+N)}^{(M+N)} X_k e^{ik\omega t}, \tag{7}$$

where,

$$X_k = \sum_{m=-M}^{M} U_m V_{(k-m)}, \tag{8}$$

and $V_{(k-m)} = 0$ for any $|k - m| > N$. Thus, the convolution theorem yields a Fourier series with a higher order of truncation than the original ansatz, which had only $H$ harmonics. To stay within the original ansatz, we truncate all higher harmonics in the convolution, and effectively set,

$$x(t) \approx \sum_{k=-M}^{M} X_k e^{ik\omega t}, \tag{9}$$

where $X_k$ is given by eqn. (8), and $M$ is either $H$ or $H - 1$ depending on the quadratic term being considered. Now, substituting (4) in eqn. (1) – (3) and equating to (6), we obtain the set of equations to be solved using HB. We can simplify these equations as follows starting with eqn. (1).

$$\begin{aligned} \frac{d\sigma_{11,H}}{dt} + \frac{\sigma_{11,H}}{\lambda} &= \sum_{k=-(H-1)}^{(H-1)} A_{2k} \left(i2k\omega\right) e^{i2k\omega t} + \frac{1}{\lambda} \sum_{k=-(H-1)}^{(H-1)} A_{2k} e^{i2k\omega t} \\ &= \sum_{k=-(H-1)}^{(H-1)} \left(i2k\omega + \frac{1}{\lambda}\right) A_{2k} e^{i2k\omega t} \end{aligned} \tag{10}$$

and

$$\sigma_{11,H}^2+\sigma_{12,H}^2=\left(\sum_{p=-(H-1)}^{(H-1)}A_{2p}e^{i2p\omega t}\right)\left(\sum_{q=-(H-1)}^{(H-1)}A_{2q}e^{i2q\omega t}\right)+$$
$$\left(\sum_{p=-H}^{(H-1)}C_{2p+1}e^{i(2p+1)\omega t}\right)\left(\sum_{q=-H}^{(H-1)}C_{2q+1}e^{i(2q+1)\omega t}\right)$$
$$=\sum_{p=-(H-1)}^{(H-1)}\sum_{q=-(H-1)}^{(H-1)}A_{2p}A_{2q}e^{i2(p+q)\omega t}+\sum_{p=-H}^{(H-1)}\sum_{q=-H}^{(H-1)}C_{2p+1}C_{2q+1}e^{i(2p+2q+2)\omega t}. \quad (11)$$

Also,

$$2\dot{\gamma}\sigma_{12,H}=\gamma_0\omega\left(e^{i\omega t}+e^{-i\omega t}\right)\sum_{r=-H}^{(H-1)}C_{2r+1}e^{i(2r+1)\omega t}$$
$$=\gamma_0\omega\sum_{r=-H}^{(H-1)}C_{2r+1}\left(e^{i(2r+2)\omega t}+e^{i2r\omega t}\right). \quad (12)$$

Combining eqns. (10) – (12), eqn. (1) transforms to

$$\sum_{k=-(H-1)}^{(H-1)}\left[\left(i2k\omega+\frac{1}{\lambda}\right)A_{2k}+\frac{\alpha}{\lambda G}\sum_{p=-(H-1)}^{(H-1)}A_{2p}A_{2(k-p)}+\right.$$
$$\left.\frac{\alpha}{\lambda G}\sum_{p=-H}^{(H-1)}C_{2p+1}C_{2(k-p)-1}-\gamma_0\omega\left(C_{2k-1}+C_{2k+1}\right)\right]e^{i2k\omega t} \quad (13)$$
$$=\sum_{k=-(H-1)}^{(H-1)}R_k^{11}e^{i2k\omega t}.$$

Similarly, eqn. (2) transforms to

$$\sum_{k=-(H-1)}^{(H-1)}\left[\left(i2k\omega+\frac{1}{\lambda}\right)B_{2k}+\frac{\alpha}{\lambda G}\sum_{p=-(H-1)}^{(H-1)}B_{2p}B_{2(k-p)}+\right.$$
$$\left.\frac{\alpha}{\lambda G}\sum_{q=-H}^{(H-1)}C_{2p+1}C_{2(k-q)-1}\right]e^{i2k\omega t}=\sum_{k=-(H-1)}^{(H-1)}R_k^{22}e^{i2k\omega t}. \quad (14)$$

Following the same approach, the terms of eqn. (3) can be simplified as,

$$\begin{aligned}\frac{d\sigma_{12,H}}{dt}+\frac{\sigma_{12,H}}{\lambda}&=\sum_{k=-H}^{(H-1)}C_{2k+1}\left(i\left(2k+1\right)\omega\right)e^{i(2k+1)\omega t}+\frac{1}{\lambda}\sum_{k=-H}^{(H-1)}C_{2k+1}e^{i(2k+1)\omega t}\\&=\sum_{k=-H}^{(H-1)}\left(i\left(2k+1\right)\omega+\frac{1}{\lambda}\right)C_{2k+1}e^{i(2k+1)\omega t}\end{aligned}\tag{15}$$

and

$$\begin{aligned}\left(\sigma_{11,H}+\sigma_{22,H}\right)\sigma_{12,H}&=\left(\sum_{p=-H}^{(H-1)}C_{2p+1}e^{i(2p+1)\omega t}\right)\left(\sum_{q=-(H-1)}^{(H-1)}\left(A_{2q}+B_{2q}\right)e^{i2q\omega t}\right)\\&=\sum_{p=-H}^{(H-1)}\sum_{q=-(H-1)}^{(H-1)}C_{2p+1}\left(A_{2q}+B_{2q}\right)e^{i(2p+2q+1)\omega t}.\end{aligned}\tag{16}$$

Also

$$\begin{aligned}\dot{\gamma}\sigma_{22,H}&=\frac{\gamma_0\omega}{2}\left(e^{i\omega t}+e^{-i\omega t}\right)\sum_{r=-(H-1)}^{(H-1)}B_{2r}e^{i2r\omega t}\\&=\frac{\gamma_0\omega}{2}\sum_{r=-(H-1)}^{(H-1)}B_{2r}\left(e^{i(2r+1)\omega t}+e^{i(2r-1)\omega t}\right).\end{aligned}\tag{17}$$

In addition,

$$G\dot{\gamma}=\frac{G\gamma_0\omega}{2}\left(e^{i\omega t}+e^{-i\omega t}\right).\tag{18}$$

Using eqn. (15) – (18), eqn. (3) becomes,

$$\begin{aligned}\sum_{k=-H}^{(H-1)}\Bigg[\left(i\left(2k+1\right)\omega+\frac{1}{\lambda}\right)C_{2k+1}+\frac{\alpha}{\lambda G}\sum_{p=-H}^{(H-1)}C_{2p+1}\left(A_{2(k-p)}+B_{2(k-p)}\right)&\\-\frac{\gamma_0\omega}{2}\left(B_{2k}+B_{2k+2}\right)-\frac{G\gamma_0\omega}{2}\delta_{|2k+1|1}\Bigg]e^{i(2k+1)\omega t}&\\=\sum_{k=-H}^{(H-1)}R_k^{12}e^{i(2k+1)\omega t}.&\end{aligned}\tag{19}$$

where $\delta_{|2k+1|1}$ respresents the Kronecker delta function which is unity only for $k=-1$ or $k=0$, and zero otherwise. Equating the terms on both sides for eqn. (13), (14) and (19), we obtain

$2H-1, 2H-1$ and $2H$ nonlinear equations respectively.

$$R_k^{11} = \left(i2k\omega + \frac{1}{\lambda}\right) A_{2k} + \frac{\alpha}{\lambda G} \sum_{p=-(H-1)}^{(H-1)} A_{2p} A_{2(k-p)} + \frac{\alpha}{\lambda G} \sum_{p=-H}^{(H-1)} C_{2p+1} C_{2(k-p)-1} - \gamma_0 \omega \left(C_{2k-1} + C_{2k+1}\right) = 0, \tag{20}$$

$$R_k^{22} = \left(i2k\omega + \frac{1}{\lambda}\right) B_{2k} + \frac{\alpha}{\lambda G} \sum_{p=-(H-1)}^{(H-1)} B_{2p} B_{2(k-p)} + \frac{\alpha}{\lambda G} \sum_{q=-H}^{(H-1)} C_{2p+1} C_{2(k-q)-1} = 0, \tag{21}$$

$$R_k^{12} = \left(i\left(2k+1\right)\omega + \frac{1}{\lambda}\right) C_{2k+1} + \frac{\alpha}{\lambda G} \sum_{p=-H}^{(H-1)} C_{2p+1} \left(A_{2(k-p)} + B_{2(k-p)}\right) - \frac{\gamma_0 \omega}{2} \left(B_{2k} + B_{2k+2}\right) - \frac{G\gamma_0\omega}{2} \delta_{|2k+1|1} = 0. \tag{22}$$

We solve the system of $(6H-2)$ nonlinear equations, one for each of the $k$th harmonics, given by eqn. (20), (21) and (22). The system is solved for the Fourier coefficients $A_{2k}, B_{2k}$ and $C_{2k+1}$, with $\alpha, \lambda$ and $G$ as system parameters, and $\gamma_0$ and $\omega$ controlling the external forcing function. In these formulae, we set $A_{2k} = 0$ and $B_{2k} = 0$ for any $|2k| > 2H$, and $C_{2k+1} = 0$ for any $|2k+1| > (2H+1)$.
